# Supplementary material for: SCLib: A Practical and Lightweight Defense against Component Hijacking in Android Applications
Source: arXiv:1801.04372 source file (2018-01-13)
Supplement: Supplementary file 1 [file appendix.tex]

\section*{Appendix}
\appendix
\section{Supplementary Tables}
\label{sec:appendix1}

In this section, we provide two supplementary tables for the contents in \mysec\ref{sec:other} and \mysec\ref{sec:tenapps}.
Specifically, Table~\ref{tab:entryfuncs} lists the component entry functions that need to be intercepted, organized by different component types and IPC call APIs.
A short description of these entry functions has been given in \mysec\ref{sec:other}, in the reverse order of component types.
On the other hand, Table~\ref{tab:dataset} presents the raw statistic data of ten open source apps measured in \mysec\ref{sec:tenapps}.
